# Supplementary material for: Scalar fields on fluctuating hyperbolic geometries
Source: arXiv:2112.00927 source file (2021-12-02)
Supplement: Supplementary file 1 [file appendix.tex]

\appendix
\section{Formulating the action}

Action for the pure gravity,
\begin{equation}
    S &=-\kappa_0 N_0 +\kappa_2 N_2
\end{equation}

Using the relation of the total number of nodes, triangles and boundary length of a disk,
\begin{equation}
   N_0=(N_2+N_{0\partial}+2)/2
\end{equation}
and rescaling the coupling constants, we obtain the action for the disk simulation in terms of the boundary length and the total number of 2-simplices
\begin{equation}
    S &=-\kappa_0 N_{0\partial} +\kappa_2 N_2.
\end{equation}

For simulation purpose, it could be convenient to just use the volume of the sphere ($N_{2,S}$) with the marked node. Note the relation of the volume of the sphere and the disk in the simulation, $N_{2,S}=N_{2,D}+N_{0\partial}$. Thus the equation can be written in terms of total number simplices in the sphere and the length of the boundary with another rescaling of the boundary cosmological constant term.

\begin{equation}
    S &=-\kappa_0 N_{0\partial} +\kappa_2 N_{2,S}.
\end{equation}

Further we introduce a volume tuning term and the coordination-constrainting term,
\begin{equation}
    S &= \gamma(N_{2,S}-V)^2 + \sum_i \beta(q_i -7)^2
\end{equation}

Change in the action in the boundary cosmological constant term,
\begin{equation}
    \Delta S_{0\partial}= -\kappa_{0\partial} \Delta N_{0\partial}.
\end{equation}

There is no contribution of this term from the bulk moves. For insertion (deletion) of node at boundary, $\Delta N_{0\partial}=1 (-1)$. For link flip at boundary that increases (decreases) the disk area $\Delta N_{0\partial}=1$ $(-1)$.

Change in the action in the sphere volume term,
\begin{equation}
    \Delta S_2 = \kappa_2 \Delta N_{2,S}.
\end{equation}

For Pachner moves of node insertion, link-flip and node deletion, $\Delta N_{2,S}=(1,0,1)$.
